# Supplementary material for: Progressive trajectory matching for medical dataset distillation
Source: arXiv:2403.13469 source file (2024-03-20)
Supplement: Supplementary file 1 [file 6_Appendix.tex]

\chensays{we can create another supp.tex for the appendix for now. because it is a bit difficult to view the whole 7-page main submission.}

\section{Appendix}

\subsection{Hyper-parameters Analysis}
%\chensays{gaussian window, learning rate, temporal parameters; }
we conduct a detailed analysis of the hyper-parameters employed in our method, and our goal is to gain a deeper understanding of the impact of hyper-parameters on experimental results by systematically adjusting and analyzing them.

\textbf{Number of Expert Trajectories.}
We evaluate our proposed method with different number of expert trajectories, and the results are shown in Table~\ref{table_4}.
It can be observed that our method performs better than the baseline methods in all aspects, and as the number of expert trajectories increases, our method can achieve a certain improvement. This indicates that our method can better utilize the generalization and diversity brought by the majority of expert trajectories, while the baseline methods do not capture the core information brought by expert trajectories well due to their unstable trajectory matching pattern0
%\textbf{Distillation Frequency per Epoch Step.}
%We also evaluate our proposed method with different distillation frequency per epoch step, and the results are shown in  Table~\ref{table_5}.

\begin{table}
\centering
\small 
\caption{Comparison of the stability performances to other trajectory matching methods as the number of expert trajectories decreases in the PATHMNIST.}
\label{table_4}
 
\resizebox{1.0\linewidth}{!}{
\begin{tabular}{c|cccc}
\hline & \multicolumn{4}{|c}{ Number of Expert Trajectories } \\
Method & 10 & 30 & 50 & 100 \\
\hline
MTT & $48.62 \pm 0.02$ & $49.16 \pm 0.02$ & $46.82 \pm 0.03$ & $50.86 \pm 0.02$ \\
FTD & $53.93 \pm 0.01$ & $55.76 \pm 0.01$ & $54.82 \pm 0.01$ & $53.47 \pm 0.02$ \\
OUR & $\mathbf{60.35} \pm \mathbf{0.02}$ & $\mathbf{63.47} \pm \mathbf{0.01}$ & $\mathbf{65.65} \pm \mathbf{0.01}$ & $\mathbf{67.01} \pm \mathbf{0.01}$ \\
\hline
\end{tabular}
}
\end{table}

\begin{comment}
\begin{table}
\centering
\small 
\caption{Comparison of the stability performances to other trajectory matching methods as the number of expert trajectories decreases in the PATHMNIST.}
\label{table_4}
 
\resizebox{1.0\linewidth}{!}{
\begin{tabular}{c|cccc}
\hline & \multicolumn{4}{|c}{ Distillation Frequency per Epoch Step } \\
Dataset & 20 & 60 & 80 & 120\\
\hline
COVID19-CXR & $xxx \pm xxx$ & $xxx \pm xxx$ & $66.18 \pm 0.02$ & $xxx \pm xxx$ \\
BREAST-ULS & $61.27 \pm 0.03$ & $64.41 \pm 0.02$ & $65.37 \pm 0.02$ & $64.94 \pm 0.02$ \\
SKIN-HAM & $xxx \pm xxx$ & $xxx \pm xxx$ & $51.19 \pm 0.02$ & $xxx \pm xxx$ \\
PathMNIST & $63.93 \pm 0.01$ & $66.29 \pm 0.01$ & $67.01 \pm 0.01$ & $65.43 \pm 0.01$ \\
OCTMNIST & $45.8 \pm 0.02$ & $47.46 \pm 0.03$ & $49.59 \pm 0.03$ & $48.80 \pm 0.02$ \\
ORGAN3D & $52.07 \pm 0.01$ & $55.16 \pm 0.01$ & $56.28 \pm 0.01$ & $54.23 \pm 0.01$ \\
\hline
\end{tabular}
}
\end{table}
\end{comment}

\begin{figure}[h]
  \includegraphics[width=3.45in]{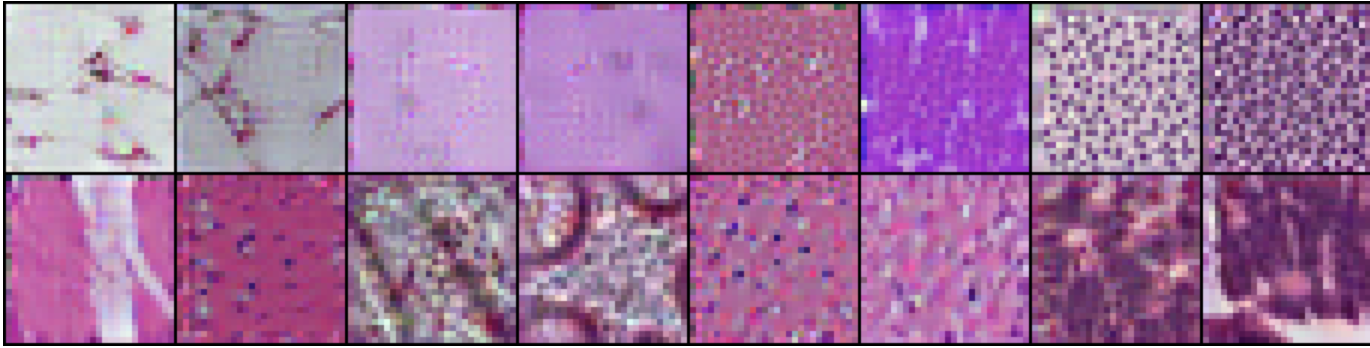}
  \includegraphics[width=3.45in]{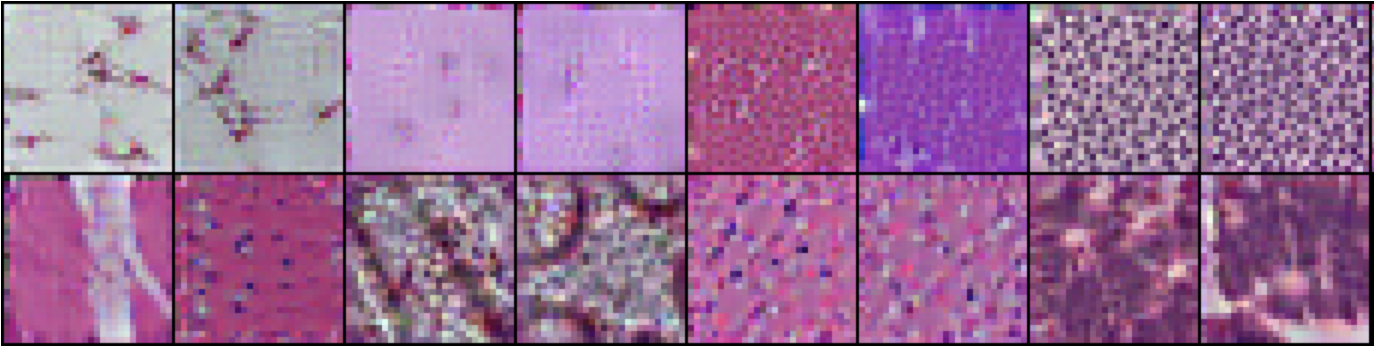}
  \includegraphics[width=3.45in]{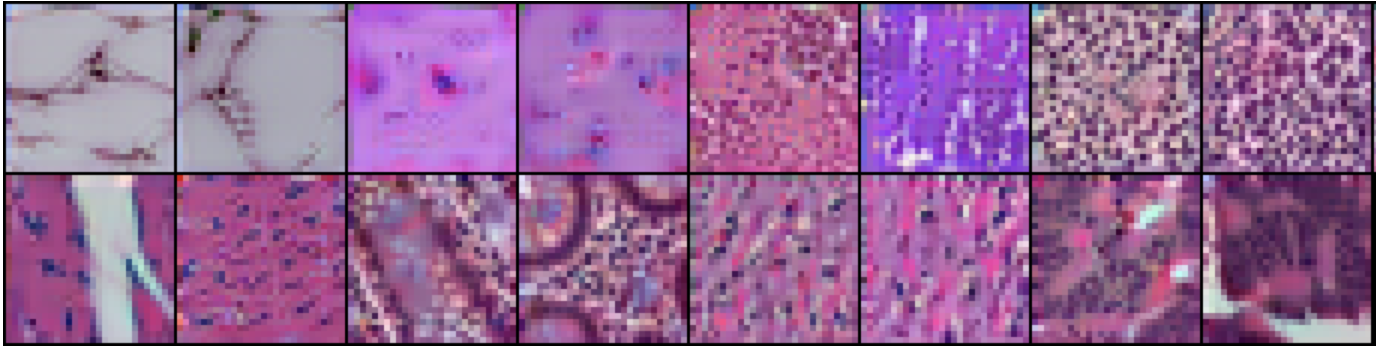}
  \includegraphics[width=3.45in]{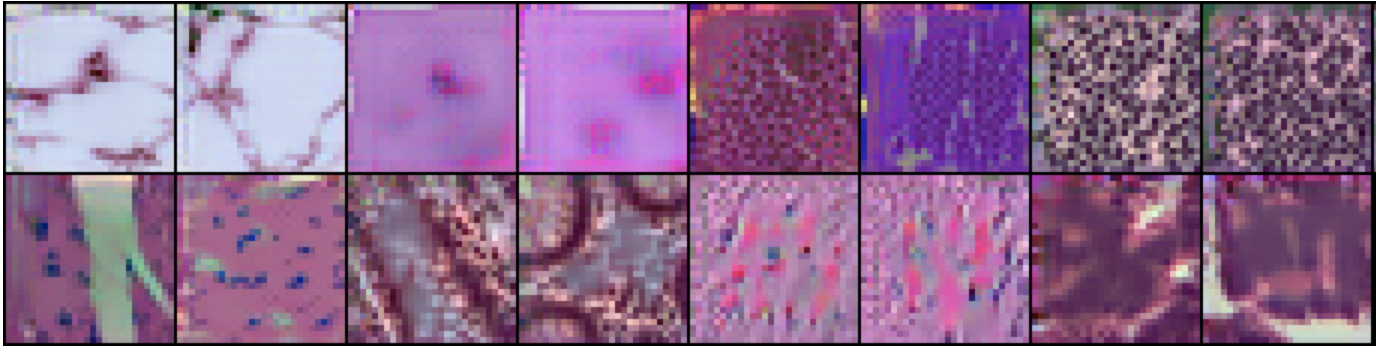}
 \caption{(a) our; (b) our with overlap; (c) ftd; (d) mtt;}
 \label{fig:0}
\end{figure}
